# Supplementary material for: Weakly Supervised Point Cloud Segmentation via Conservative Propagation of Scene-level Labels
Source: arXiv:2312.06799 source file (2025-06-13)
Supplement: Supplementary file 1 [file supp_qualitative.tex]

\newcommand{\suppqualiscannetimagewidth}{4.5cm}
\newcommand{\suppqualiscannetrowimage}[2]{%
    \includegraphics[width=\suppqualiscannetimagewidth, trim={0pt 0pt 0pt 0pt}, clip]{assets/supp_qualitative/Extra_Fig_3_#1_#2.png}%
}

\newcommand{\suppquali}{
    \begin{tikzpicture}[
        >=stealth',
        overlay/.style={
          anchor=south west, 
          draw=black,
          rectangle, 
          line width=0.8pt,
          outer sep=0,
          inner sep=0
        }
    ]
        \matrix[
        matrix of nodes, 
        column sep=0pt, 
        row sep=0pt, 
        ampersand replacement=\&, 
        inner sep=0, 
        outer sep=0
        ] (main) {
            \suppqualiscannetrowimage{e}{CAM} \&
            \suppqualiscannetrowimage{e}{Ours} \&
            \suppqualiscannetrowimage{e}{Ours_Retrain} \&
            \suppqualiscannetrowimage{e}{GT} \\
            \suppqualiscannetrowimage{f}{CAM} \&
            \suppqualiscannetrowimage{f}{Ours} \&
            \suppqualiscannetrowimage{f}{Ours_Retrain} \&
            \suppqualiscannetrowimage{f}{GT} \\
            \suppqualiscannetrowimage{h}{CAM} \&
            \suppqualiscannetrowimage{h}{Ours} \&
            \suppqualiscannetrowimage{h}{Ours_Retrain} \&
            \suppqualiscannetrowimage{h}{GT} \\
            \suppqualiscannetrowimage{g}{CAM} \&
            \suppqualiscannetrowimage{g}{Ours} \&
            \suppqualiscannetrowimage{g}{Ours_Retrain} \&
            \suppqualiscannetrowimage{g}{GT} \\
        };
        \node[below=0.1em of main-4-1.south, align=center, anchor=north]{CAM~\cite{Wei_2020_CVPR}};
        \node[below=0.1em of main-4-2.south, align=center, anchor=north]{\textbf{Ours}};
        \node[below=0.1em of main-4-3.south, align=center, anchor=north]{\textbf{Ours}$^\star$};
        \node[below=0.1em of main-4-4.south, align=center, anchor=north]{Ground Truth};
    \end{tikzpicture}
}

\begin{figure*}[t]
  \resizebox{\linewidth}{!}{\suppquali}
  \caption{
    \textbf{Additional qualitative results} -- We show additional qualitative results of our and CAM~\cite{Wei_2020_CVPR}~methods.  We denote \textbf{Ours}$^\star$ as training with bootstrapping. 
  }
  \label{fig:supp_scannet_quali}
\end{figure*}
